# Supplementary material for: Learning Signal-Agnostic Manifolds of Neural Fields
Source: arXiv:2111.06387 source file (2021-11-11)
Supplement: Supplementary file 1 [file supplement.tex]

\documentclass{article} %
\usepackage[nonatbib]{neurips_2021}
\usepackage[numbers,sort&compress]{natbib}
\usepackage[utf8]{inputenc} %
\usepackage[T1]{fontenc}    %
\input{packages}
\input{macros}
\input{math_commands}
\usepackage{hyperref}
\usepackage{url}
\usepackage{caption}
\captionsetup{font=small}

\title{Learning Signal-Agnostic Implicit Manifolds Appendix}

\author{Antiquus S.~Hippocampus, Natalia Cerebro \& Amelie P. Amygdale \thanks{ Use footnote for providing further information
about author (webpage, alternative address)---\emph{not} for acknowledging
funding agencies.  Funding acknowledgements go at the end of the paper.} \\
Department of Computer Science\\
Cranberry-Lemon University\\
Pittsburgh, PA 15213, USA \\
\texttt{\{hippo,brain,jen\}@cs.cranberry-lemon.edu} \\
\And
Ji Q. Ren \& Yevgeny LeNet \\
Department of Computational Neuroscience \\
University of the Witwatersrand \\
Joburg, South Africa \\
\texttt{\{robot,net\}@wits.ac.za} \\
\AND
Coauthor \\
Affiliation \\
Address \\
\texttt{email}
}

\begin{document}

\renewcommand{\thesection}{A.\arabic{section}}
\renewcommand{\thefigure}{A\arabic{figure}}
\setcounter{section}{0}
\setcounter{figure}{0}

\appendix
\input{text/appendix}

{\small
\bibliographystyle{plainnat}
\bibliography{reference,manifold}
}

\end{document}
